# Supplementary material for: Active Connectivity Fundamentals for TSCH Networks of Mobile Robots
Source: arXiv:2201.08202 source file (2022-01-20)
Supplement: Supplementary file 1 [file Appendix.tex]

\section{Appendix}

\begin{figure*}[htp]

\centering
\includegraphics[width=.33\textwidth]{figures/throughput[1,3]_AC_linear_all.pdf}\hfill
\includegraphics[width=.33\textwidth]{figures/downtime[1,3]_AC_linear_all.pdf}\hfill
\includegraphics[width=.33\textwidth]{figures/distance[1,3]_AC_linear_all.pdf}
\caption{[1,3] linear acceleration, linear brake}

\centering
\includegraphics[width=.33\textwidth]{figures/throughput[1,3]_ACNOGPS_linear_all.pdf}\hfill
\includegraphics[width=.33\textwidth]{figures/downtime[1,3]_ACNOGPS_linear_all.pdf}\hfill
\includegraphics[width=.33\textwidth]{figures/distance[1,3]_ACNOGPS_linear_all.pdf}
\caption{[1,3] linear acceleration, linear brake}

\end{figure*}
